# Supplementary material for: Identifying features predictive of faculty integrating computation into physics courses
Source: arXiv:1810.07859 ancillary file (2019-01-23)
Supplement: Supplementary file 1 [file Supplemental_material.pdf]

# Supplemental Material

## I. THE RANDOM FOREST ALGORITHM

### A. Decision tree learning

Random forests have their roots in the decision tree learning [1]. Decision tree learning uses a set of binary decisions to develop a model for the data set. For our purposes, we focus on classification trees where the object of the model is a class label (i.e., a particular categorical outcome). The decision tree algorithm is provided with the classes and the data that should predict the classes (i.e., input variables). Conceptually, the decision tree algorithm searches the input variables for the one that best segregates the data into separate classes. That choice of "best" can be user specified, but if left to the algorithm, it will be the variable for which a majority of members of a class appear on one side of the decision (termed "branch") and not on the other side. For input variables that are continuous data, the algorithm further decides on the binary decision that best splits the data. For example, if "age $<$ 55" was the binary decision, the algorithm both chose "age" as the input variable and "55" as the cut-off. The algorithm continues to make these decisions, splitting the data into more and more branches until all branches terminate in a single class (termed "leaves") or until a user-specified level. Tracing the path back from any leaf (single class or multiclass) to the starting point shows all the decisions that were made to obtain that leaf. In this sense, decision tree learning is a glass-box algorithm – a researcher can see every step along the path.

Although the researcher can view all parts of the model and how it was constructed, any single decision tree is strongly tied to the data used to construct it. This leads to overfitting of the data [1, 2]. That is, the decision tree algorithm can produce a model that exactly provides unique classifications for the data it is given. As such, applying that model to predict classes in a new data set will often produce false predictions as the model was so strongly tied to the initial data set on which it was trained. Overfitting is a common problem in machine learning techniques where a single analysis is conducted [3]. To deal with this, some decisions trees are pruned [4] – reduced to a smaller size by removing leaves that predict only small classes. However, as computational time has become less expensive, ensemble methods that develop a series of models from random selections of data are a more common method for combating overfitting [5]. The Random Forest algorithm is one such ensemble method, which grows out of decision tree learning.

### B. Random decision trees

A Random Forest is grown from a set of random decision trees and stems from a technique known as "tree bagging." Tree bagging, or simply bagging, refers to running the decision tree algorithm a specified number of times on a random selection of data with replacement [6]. Data selected to be used in the algorithm is "bagged." Each time the algorithm runs, it produces a decision tree from a randomly selected set of data. The input variables are scored based on how well they classify the data. Those that continually classify well earn higher scores, while those that do not are given lower scores. The result is a set of input variables that have been tested on a variety of data sets so that those input variables that are most important for classification can be found. Random forests use the bagging technique, but also randomly select a subset of input variables [7]. That is, data to develop the Random Forest model are randomly selected and only a subset of input variables (again, randomly chosen) are used in the classification. The same scoring procedure for these input variables is used. Both the bagging and Random Forest algorithms combat overfitting by leveraging random selection as opposed to pruning. Conceptually, when randomly sampling data, the trained model will sometimes produce a good model and at other times it will not. By checking the quality of each decision tree model after each run, the algorithms ensure that consistently-appearing predictors from good models are carried into the complete bagging or Random Forest model and others are not. Due to randomly selecting a subset of the input variables in addition to a bootstrapped sample of the data, Random Forests have been shown to have significant advantage over bagging alone [8].

### C. Tuning Random Forest Parameters

Random forests have two tuning parameters that can be adjusted to obtain a reliable model, $n_{in}$ – the number of input variables selected at random, and $n_{trees}$ – the number of trees in the forest. A review of how $n_{in}$ can affect the predictions of a Random Forest has been conducted by Svetnik et al. [9]. For a variety of choices of $n_{in}$, Svetnik et al. compared error rates (fraction of false positives and false negatives) predictions and found that for most choices

| | | Known Classes | |
|---|---|---|---|
| | | Yes | No |
| **Model** | Yes | $N_{TP}$ | $N_{FP}$ |
| **Predicts** | No | $N_{FN}$ | $N_{TN}$ |

FIG. 1: The confusion matrix counts the number of each predicted classification by the model and compares that to the what the data indicates. In this case, a two class system with binary classifications leads to a 2 x 2 matrix. For $M$ classes, the matrix continues to be square and grows to be $M$ x $M$.

of $n_{in}$ error rates were well maintained between 20-25%. For lower $n_{in}$, the model does not develop enough robust comparisons between different input variables to be reliable leading to slightly elevated error rates. While for higher $n_{in}$, the model overfits the training data leading to higher scores for less important variables, which again produce slightly higher error rates. For a given number of input variables, $N$, Svetnik et al. suggested $n_{in}$ include $N/2$, $N/4$, and $\sqrt{N}$ where each is rounded up or down to the nearest integer. They tested these suggested choices and found that all choices produce similar error rates even as the number of input variables is varied between 3 and 100. After 100 variables, the choice $n_{in} = \sqrt{N}$ performs slightly better than the other choices, but only marginally so (2% difference in error rates).

The number of trees in the forest, $n_{trees}$, describes the number of times that the algorithm randomly selects data and input variables to perform the classification task. Here, more is better, but only up to a point, after which adding addition trees does not improve the classification. There is no penalty for running the algorithm many times besides wasting computational resources. An estimate of the model's performance for a given number of trees is the Out-Of-Bag error (OOB error). When the algorithm selects data to train, it leaves some data "out of the bag." For any given tree in the forest, we can predict the classifications for the data left out of the bag. The error rate associated with that prediction is an estimate of the Out-Of-Bag error for that tree. The estimate for the total OOB error is the average across all the trees. In their work, Svetnik et al., found that OOB error stabilized when $n_{trees} > 10^2$. For 3 orders of magnitude beyond that the OOB error remained flat at 0.2, that they found a ∼20% average misclassification of data left out of the bag for any number of trees from $10^2 - 10^5$.

It is common to determine the "best" parameters by using a grid search [10]. Here, a number of random forests are constructed with different combinations of $n_{in}$ and $n_{trees}$ to find the combination with the strongest validation scores. Typically, one performs a coarse-grain search allowing the tunable parameters to vary greatly. This is much like searching for the appropriate order of magnitude for each parameter. Once a reasonable range is found for each parameter, a finer-grain search is performed within the bounds determined from the coarse grained search. This search can continue *ad infinitum*, but it is typically only done until reasonable estimates of the "best" parameters are found given the expected error and available computational time.

## II. VALIDATING THE RANDOM FOREST MODEL

A Random Forest will develop a model of data, but that does not always mean that model is meaningful. Moreover, because that model is developed from a random selection of data and input variables, individual trees in the model might be terrible predictors. By abiding by suggested parameter choices [9], one can be somewhat confident in the model. However, additional validation of the model can be conducted to be able to provide evidence of that confidence. These metrics and the associated curves are developed from how well the model predicts classifications of the test data – that is, the data that was not used to train the model.

### A. Confusion Matrix

The simplest tool for understanding how well the Random Forest model predicts classifications in the new data set is the confusion matrix. Most other measures associated with validity of the model are derived from the confusion matrix. Conceptually, the confusion matrix keeps track of true positives ($N_{TP}$), true negatives ($N_{TN}$), false positives ($N_{FP}$), and false negatives ($N_{FP}$). The sum of all these measures is the total number of observations in the data set that is being tested ($N_{test}$).

$$N_{test} = N_{TP} + N_{TN} + N_{FP} + N_{FN} \tag{1}$$

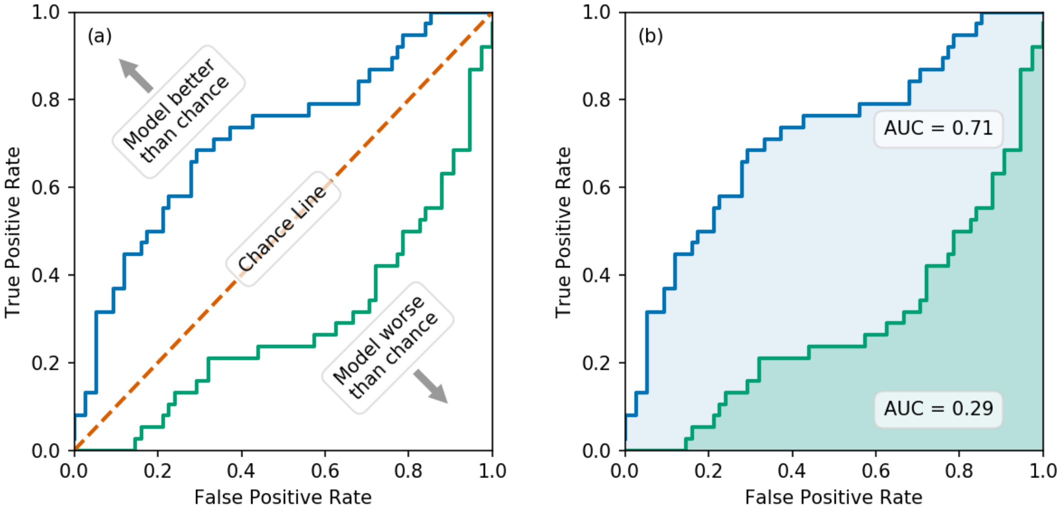


FIG. 2: (a) Sample receiver operating characteristic (ROC) curves that demonstrate two models: one that is better than chance (blue) and one that is worse than chance (green). These ROC curves are plotted along with the chance line (orange dotted). Models that are demonstrably better than chance have ROC curves that tend towards the upper-left corner of the space as the arrow indicates. Models that are worse than chance tend towards the bottom-right corner. (b) For both models, the area under the ROC curves (AUC) are shown (blue and green shading) and computed. AUC provides a measure of the quality of the model. It is indicative of the probability of accurately classifying a random sample from the data.

For a two class system (e.g., Yes/No), these values can be organized into the 2 x 2 matrix where the columns describe the known classes in the data set and the rows describe the classes predicted by the model (Fig. 1). The confusion matrix provides a quick check of the predictions of the Random Forest model. Essentially a good model will have strong diagonal elements, that is, high numbers of true predictions, and small off-diagonal elements, low numbers of false predictions.

### B. Associated measures

From the confusion matrix, a number of associated measures may be derived. Here we provide those that are common to report in the Random Forest literature. Additional measures exist, but are not reported here [11]. The accuracy of the model ($ACC$) is the fraction of true predictions compared to the total number of observations in the test data set,

$$ACC = \frac{N_{TP} + N_{TN}}{N_{test}}. \tag{2}$$

This accuracy of the model can vary between 0 and 1, with 0.5 being equal to chance predictions. A model that predicts worse than chance will have $ACC < 0.5$. The sensitivity, or the true positive rate ($TPR$) compares the number of predicted true positives to the total number of actual positives appearing in the test data,

$$TPR = \frac{N_{TP}}{N_{TP} + N_{FN}}. \tag{3}$$

This rate varies between 0 and 1. For a good model of the data, we expect this number to be closer to 1. The fall-out, or false positive rate ($FPR$) compares the number of predicted false positives negatives to the total number of actual negatives in the data,

$$FPR = \frac{N_{FP}}{N_{FP} + N_{TN}}. \tag{4}$$

This rate varies between 0 and 1. For a good model of the data, we expect this number to be closer to 0. Pure guessing (i.e., chance) would yield 0.5 for both of these values. Taken together, these values are plotted together for a range of discrimination thresholds in a receiver operating characteristic curve, which indicate how much better (or worse) the model is than chance.

### C. Receiver operating characteristic curve

The receiver operating characteristic curve (ROC curve) provides a visualization of the quality of a binary model [12]. In it, $TPR$ is plotted against $FPR$ for a variety of discrimination thresholds. These thresholds vary from 0 to 1 and describe the probability above which an observation is placed into one class compared to another. Conceptually, it determines, at a given probability of classification, the expected rates of true positives compared to false positives.

A sample ROC for mock data is plotted in Fig. 2(a). The chance line, in which $TPR$ and $FPR$ are equal for all thresholds, is plotted in orange. The blue curve is the ROC curve for a model that is better than chance. The humped-shaped of curve is common for good models as this shape are indicative of $TPR$ values above chance for all thresholds. On the other hand, the green curve is the ROC curve for a model that is worse than chance. This shape is characteristic as well as it is indicative of $TPR$ below chance for all thresholds.

A quantitative measure of the quality of the model is the area under the ROC curve (AUC). This measure is visually represented in Fig. 2(b) where AUC for the better than chance model is indicated by the blue and the green shading taken together. The AUC for the worse than chance model is indicated by the green shading alone. AUC is indicative of the probability that model will rank a randomly chosen positive instance higher than a randomly chosen negative one. From Fig. 2, the probability for the first model is approximately 0.71 while for the second it 0.29. AUCs above 0.7 are typically considered reasonable models with 0.8 and above considered to be good models [13]. A perfect classifier will have an area under the curve of 1 while the chance curve will have an area under the curve of 0.5.

## III. FEATURE SELECTION

One of the more useful aspects of machine learning, and of the Random Forest algorithm in particular, is the ability to determine which features are more important than other features in the data. For classification tasks, that means finding the input variables that consistently separate the results into classes. There is an analogy to regression analysis where the important input variables in a Random Forest classifier act as statistically significant correlates with the outcome variable. However, because Random Forests are not rooted in traditional statistical analysis, the important features do not arise from correlation – linear or otherwise.

Feature selection makes use of these important features to reduce the overall number of input variables needed to classify the data. This is similar to using regression models of increasing complexity to find the minimal model that explains the outcomes sufficiently. These important features can be used as the sole input variables and the resulting model can be validated using the techniques described in Sec. II. A good reduced model will maintain high accuracy, produce an ROC curve that is still above the chance line for all thresholds, and have an AUC that is similarly well above chance while using the minimum amount of features.

To determine the importance of an input variable (termed "feature importance"), the standard Random Forest algorithm (CART) continuously compares how well each input variable in a single decision tree separates the data set into classes. For the CART algorithm, the measure of how well this occurs is either the Gini impurity or the information gain, depending on user selection and choice of tool. For the simplest implementation of the Random Forest classifier, the feature importance is related to the Gini impurity ($I_G$)[7], which is the total decrease in node impurity. $I_G$ is computed for each input variable (node) and is then averaged for each input variable over all the trees in the forest. Conceptually, $I_G$ for an input variable is probability of the input variable showing up in a given class multiplied by the probability of a misclassification within that factor summed over all classes [14]. Thus the higher $I_G$ for an input variable in a given tree, the less favorable choice it is for splitting the tree. For example, a high $I_G$ input variable would not be selected as the input variable for the first branch in a given tree. For this implementation, important features are those which consistently produce the best splits for a large proportion of trees in the forest. The feature importances are often distributed normally around some mean and are reported with error that is inversely proportional to the square root number of trees in which the input variable was randomly selected for use.

## IV. BIAS AND IMPROVEMENTS

While the CART algorithm and the associated Gini-based feature selection are commonly used in Random Forest classification, both are subject to biases that for certain kinds of data (including those analyzed in this paper) can lead to inaccurate models. First, the Gini-based feature selection described above is not reliable when the input variables vary in scale of measurement or in the number of categories (possible responses)[15]. This is because variables with more categories can be split into two groups in more ways than variables with less categories can and hence, it is more likely a favorable split could be found. Furthermore, Gini-based feature importances can be biased if the variables are correlated [16]. In such cases, accuracy-based permutation variable importances can be used [17, 18]. Accuracy-based permutation variable importances are based on the idea that if a input variable is associated with the outcome variable, then permutating the input variable should break that association, and therefore, the accuracy ($ACC$) should decrease. The input variables that change the accuracy the most are then said to have the largest variable importance.

However, these accuracy based variable importances are biased when the sample is unbalanced, that is, the categories in the predicted variable do not occur in equal frequencies [19]. Janitza et al. suggest modifying the accuracy-based permutation variable importances to be based on the AUC instead of accuracy because accuracy is biased toward the majority class while the AUC is not. When applying this modification, they found that the AUC-based permutation feature importances are better able to discriminate between variables that are good predictors and variables that are poor predictors than the accuracy-based permutation feature importances are when the sample is unbalance. When the sample is balanced, they reported no significant different between the two methods.

Because the Random Forest algorithm is based off classification and regression trees (CART)[20] and CART uses the Gini impurity to determine the split points, the Random Forest algorithm itself is biased for the same reasons the Gini-based feature importance is. This bias can be corrected using conditional inference forests based on the framework proposed by Hothorn et al [15, 21]. The conditional inference forest algorithm breaks the determining the split points into two steps, unlike the Random Forest algorithm, which selects the input variable and its split point in a single step. First, algorithm tests the global null hypothesis that there is no association between any of the input variables and predicted variable at some predetermined level of significance. If this test fails, the algorithm terminates. If the null hypothesis can be rejected, the algorithm selects the input variable with the strongest association to the predicted variable as measured by its P value. The algorithm then splits the input variable into two groups that maximizes a chosen test statistic. Finally, the algorithm returns to the first step and retests the global null hypothesis and either terminates or continues with the next input variable with the highest association to the predicted variable. This revised version of the Random Forest algorithm has been found to be unbiased even when the variables vary in scale of measurement or in the number of categories provided that boostrapping is not used (subsampling must occur without replacement or the original biases are still present) [15].

### A. Determining “significant” features

While we have detailed various improvements to variable selection, none of these methods can by themselves determine whether the variables are actually important, only how important they are with respect to each other. Various approaches to determine the actual important variables have been proposed such as selecting the top 10% of the variables ordered by an importance measure [22], selecting all variables above the absolute value of the most negative importance values [8], using recursive backward elimination to select the fewest number of variables that result in an OOB rate within 1 standard error of the best OOB rate [23], generating a null distribution of each variable and then assigning a $p$-value based on the fraction of null importances greater than the actual importance value [24], and mirroring the distribution of negative importances to generate an overall null distribution for the importances and again assigning a $p$-value based on the fraction of null importances greater than the actual importance value [25]. Each of these approaches has its own benefits and problems such related to ease of implementation and computation time required and to our knowledge, there is no standard choice of procedure. As we had a limited number of negative importances and limited computational power, we used recursive backward elimination in this study. Since these “significant” factors are not determined by tests of statistical significant but rather by how much the model changes when they are removed, we refer to the selected factors as meaningful factors.

---

[1] L. Rokach and O. Maimon, *Data mining with decision trees: theory and applications* (World scientific, 2014).
[2] M. Bramer, *Principles of data mining*, vol. 180 (Springer, 2007).

[3] P. Domingos, *A few useful things to know about machine learning*, Communications of the ACM **55**, 78 (2012).

[4] H. Trevor, T. Robert, and F. JH, *The elements of statistical learning: data mining, inference, and prediction* (New York, NY: Springer, 2009).

[5] T. G. Dietterich et al., *Ensemble methods in machine learning*, Multiple classifier systems **1857**, 1 (2000).

[6] L. Breiman, *Bagging predictors*, Machine learning **24**, 123 (1996).

[7] L. Breiman, *Random forests*, Machine learning **45**, 5 (2001).

[8] C. Strobl, J. Malley, and G. Tutz, *An Introduction to Recursive Partitioning: Rationale, Application and Characteristics of Classification and Regression Trees, Bagging and Random Forests*, Psychol Methods **14**, 323 (2009), ISSN 1082-989X.

[9] V. Svetnik, A. Liaw, C. Tong, J. C. Culberson, R. P. Sheridan, and B. P. Feuston, *Random forest: a classification and regression tool for compound classification and qsar modeling*, Journal of chemical information and computer sciences **43**, 1947 (2003).

[10] J. Bergstra and Y. Bengio, *Random search for hyper-parameter optimization*, Journal of Machine Learning Research **13**, 281 (2012).

[11] Note1, in some publications, certain likelihood ratios ($LR+ = TPR/FPR$ and $LR- = FNR/TNR$), odds ratios ($LR+/LR-$), and the $F_1$ score are reported, but $ACC$, $TPR$, and $FPR$ are the most commonly reported metrics.

[12] T. Fawcett, *An introduction to roc analysis*, Pattern recognition letters **27**, 861 (2006).

[13] M. B. Arajo, R. G. Pearson, W. Thuiller, and M. Erhard, *Validation of speciesclimate impact models under climate change*, Global Change Biology **11**, 1504 (2005), https://onlinelibrary.wiley.com/doi/pdf/10.1111/j.1365-2486.2005.01000.x.

[14] M. Kirk, *Thoughtful machine learning: A test-driven approach* (" O'Reilly Media, Inc.", 2014).

[15] C. Strobl, A.-L. Boulesteix, A. Zeileis, and T. Hothorn, *Bias in random forest variable importance measures: Illustrations, sources and a solution*, BMC Bioinformatics **8**, 25 (2007), ISSN 1471-2105.

[16] K. K. Nicodemus and J. D. Malley, *Predictor correlation impacts machine learning algorithms: implications for genomic studies*, Bioinformatics **25**, 1884 (2009), ISSN 1367-4811.

[17] K. K. Nicodemus, *Letter to the Editor: On the stability and ranking of predictors from random forest variable importance measures*, Brief Bioinform **12**, 369 (2011), ISSN 1467-5463.

[18] A.-L. Boulesteix, A. Bender, J. Lorenzo Bermejo, and C. Strobl, *Random forest Gini importance favours SNPs with large minor allele frequency: impact, sources and recommendations*, Brief. Bioinformatics **13**, 292 (2012), ISSN 1477-4054.

[19] S. Janitza, C. Strobl, and A.-L. Boulesteix, *An AUC-based permutation variable importance measure for random forests*, BMC Bioinformatics **14**, 119 (2013), ISSN 1471-2105.

[20] L. Breiman, J. Friedman, C. Stone, and R. Olshen, *Classification and Regression Trees* (Taylor & Francis, 1984).

[21] T. Hothorn, K. Hornik, and A. Zeileis, *Unbiased Recursive Partitioning: A Conditional Inference Framework*, Journal of Computational and Graphical Statistics **15**, 651 (2006), ISSN 1061-8600.

[22] D. M. Reif, A. A. Motsinger-Reif, B. A. McKinney, M. T. Rock, J. E. Crowe, and J. H. Moore, *Integrated analysis of genetic and proteomic data identifies biomarkers associated with adverse events following smallpox vaccination*, Genes Immun. **10**, 112 (2009), ISSN 1476-5470.

[23] R. Daz-Uriarte and S. Alvarez de Andrs, *Gene selection and classification of microarray data using random forest*, BMC Bioinformatics **7**, 3 (2006), ISSN 1471-2105.

[24] A. Hapfelmeier and K. Ulm, *A new variable selection approach using Random Forests*, Computational Statistics & Data Analysis **60**, 50 (2013), ISSN 0167-9473.

[25] S. Janitza, E. Celik, and A.-L. Boulesteix, *A computationally fast variable importance test for random forests for high-dimensional data*, Adv Data Anal Classif pp. 1–31 (2016), ISSN 1862-5347, 1862-5355.
